# Supplementary material for: Direct interpretation of the X-ray and neutron 3D-$\Delta$PDFs of yittria stabilized zirconia
Source: arXiv:2212.10907 source file (2022-12-21)
Supplement: Supplementary file 1 [file Supplement.pdf]

# Direct interpretation of the X-ray and neutron 3D-$\Delta$PDFs of yittria stabilized zirconia

## SUPPORTING INFORMATION

Ella M. Schmidt*, Reinhard B. Neder, James D. Martin, Arianna Minelli, Marie-Hélène Lemée-Cailleau, and Andrew L. Goodwin

*E-mail: ella.schmidt@uni-bremen.de

## 1 Scanning Electron Microscopy (SEM) Energy Dispersive X-ray (EDX) analysis

A JEOL 6480 LV SEM equipped with an Oxford Instruments X-MAX80 SD X-ray detector and INCA X-ray analysis system was used to image the samples and perform the analysis using EDX. In this case the microscope was used in low vacuum mode, which a small amount of air is admitted to the specimen chamber to prevent the sample from charging. In this case a chamber pressure of 30 Pa was used and an accelerating voltage of 15 kV.

In total four spectra were taken from the specimen. The reconstructed spectrum is shown in Figure S1. Table S1 lists the results of the analysed spectra in atomic %. To estimate the composition we assume a composition $Zr_{1-x}Y_xO_{2-x/2}$ for our sample and consider the ratio of Y to Zr. With this we arrive at $x \approx 18\%$.

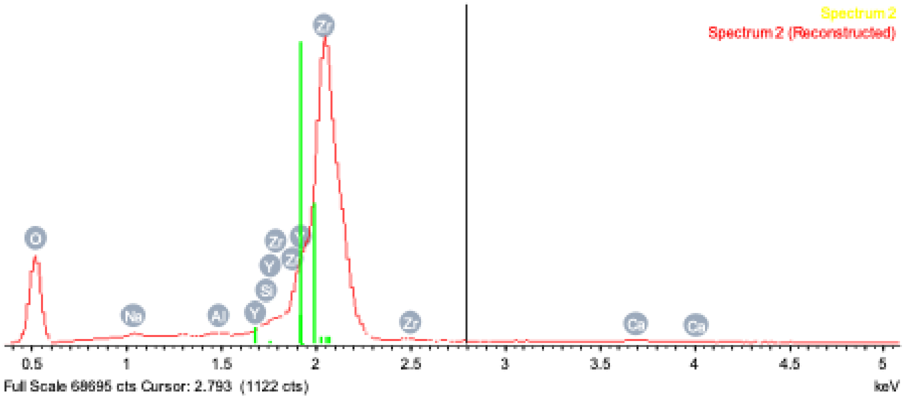


**Figure S1:** Reconstructed EDX spectrum.

| | Y | Zr | Na | Al | Si | Ca | O |
|---|---|---|---|---|---|---|---|
| Spectrum 1 | 4.9 | 22.4 | 0.5 | 0.2 | 0.5 | 0.3 | 71.1 |
| Spectrum 2 | 4.9 | 22.3 | 0.3 | 0.2 | 0.5 | 0.3 | 71.6 |
| Spectrum 3 | 4.9 | 22.4 | 0.3 | 0.2 | 0.5 | 0.3 | 71.4 |
| Spectrum 4 | 5.1 | 22.9 | 0.4 | 0.2 | 0.5 | 0.2 | 70.8 |
| Mean | 4.95(10) | 22.50(27) | 0.38(9) | 0.20(0) | 0.50(0) | 0.28(5) | 71.23(35) |

**Table S1:** Results in atomic % from EDX measurement of the specimen.

## 2 X-ray measurement

The polished specimen is shown in Figure S2. Our measured X-ray 3D-$\Delta$PDF shows a weak but clear signature at $\langle \frac{1}{2}, 0, 0 \rangle$ and therefore manifests that the oxygen displacements can be directly observed in the X-ray diffraction case and hence need to be included explicitly in any real-space and reciprocal-space modelling.

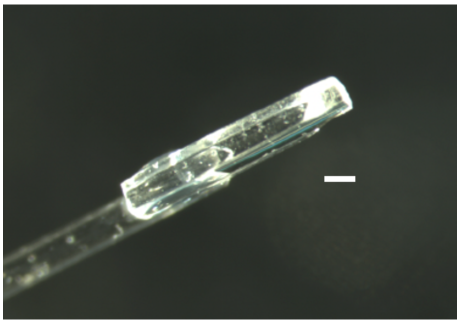

**Figure S2:** Polished crystal mounted onto glass fibre for X-ray diffraction experiments. Scale bar $\approx$ 200$\mu$m.

## 3 Comparison of the Data and the Model

Figures S3 and S4 compare selected layers fo the calculated diffuse scattering and the 3D-$\Delta$PDF from the simplistic atomistic model to the experimentally obtained data.

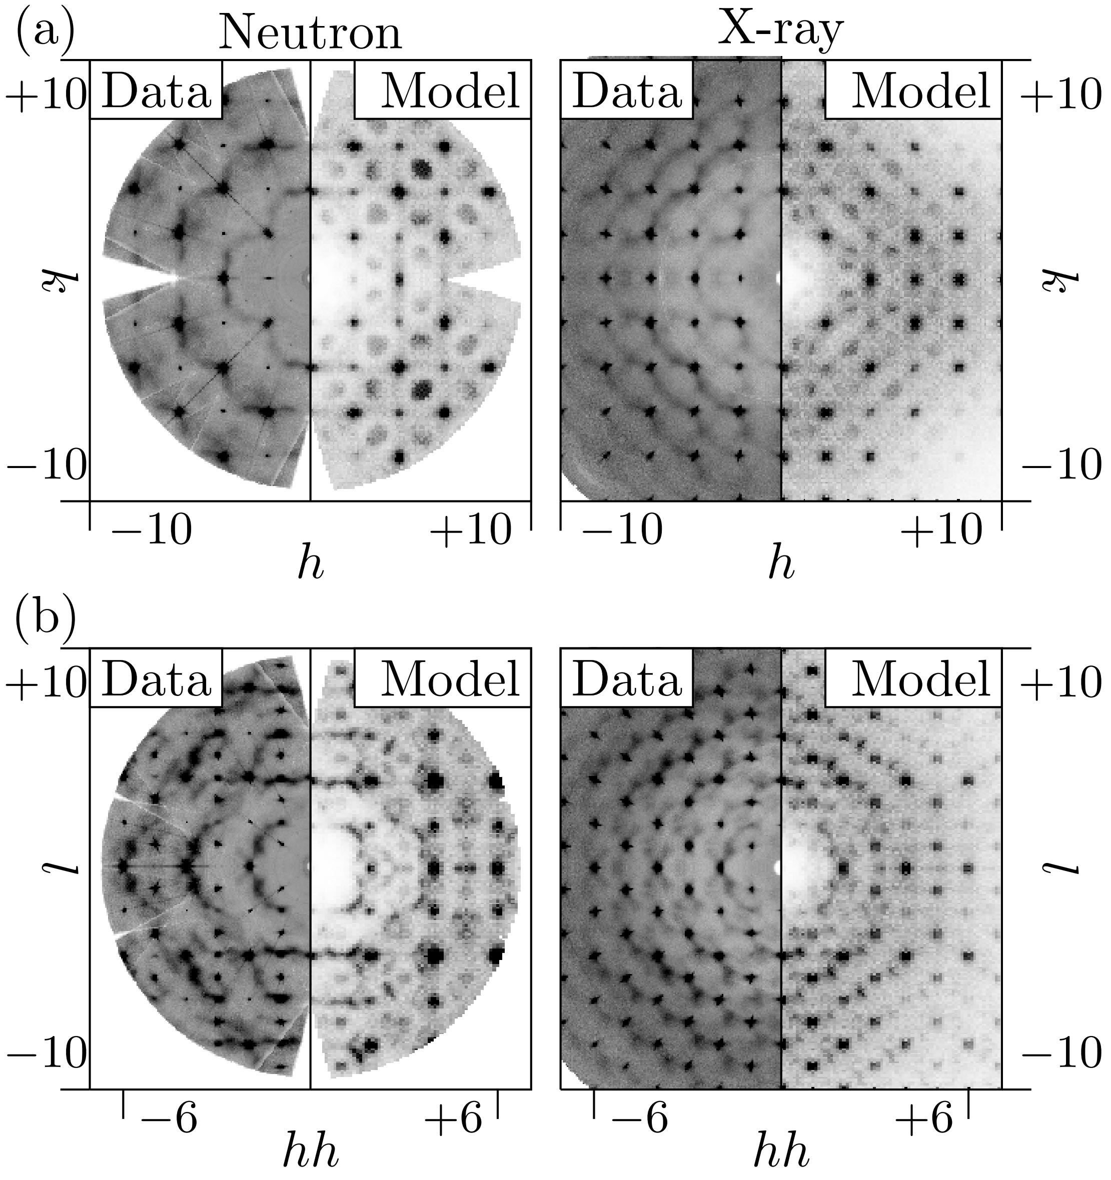


**Figure S3:** Reconstructed and symmetry averaged diffuse scattering of YSZ obtained from neutron (left) and X-ray (right) diffraction experiments compared to the results of modelling. (a) $hk0$-layer, (b) $hhl$-layer.

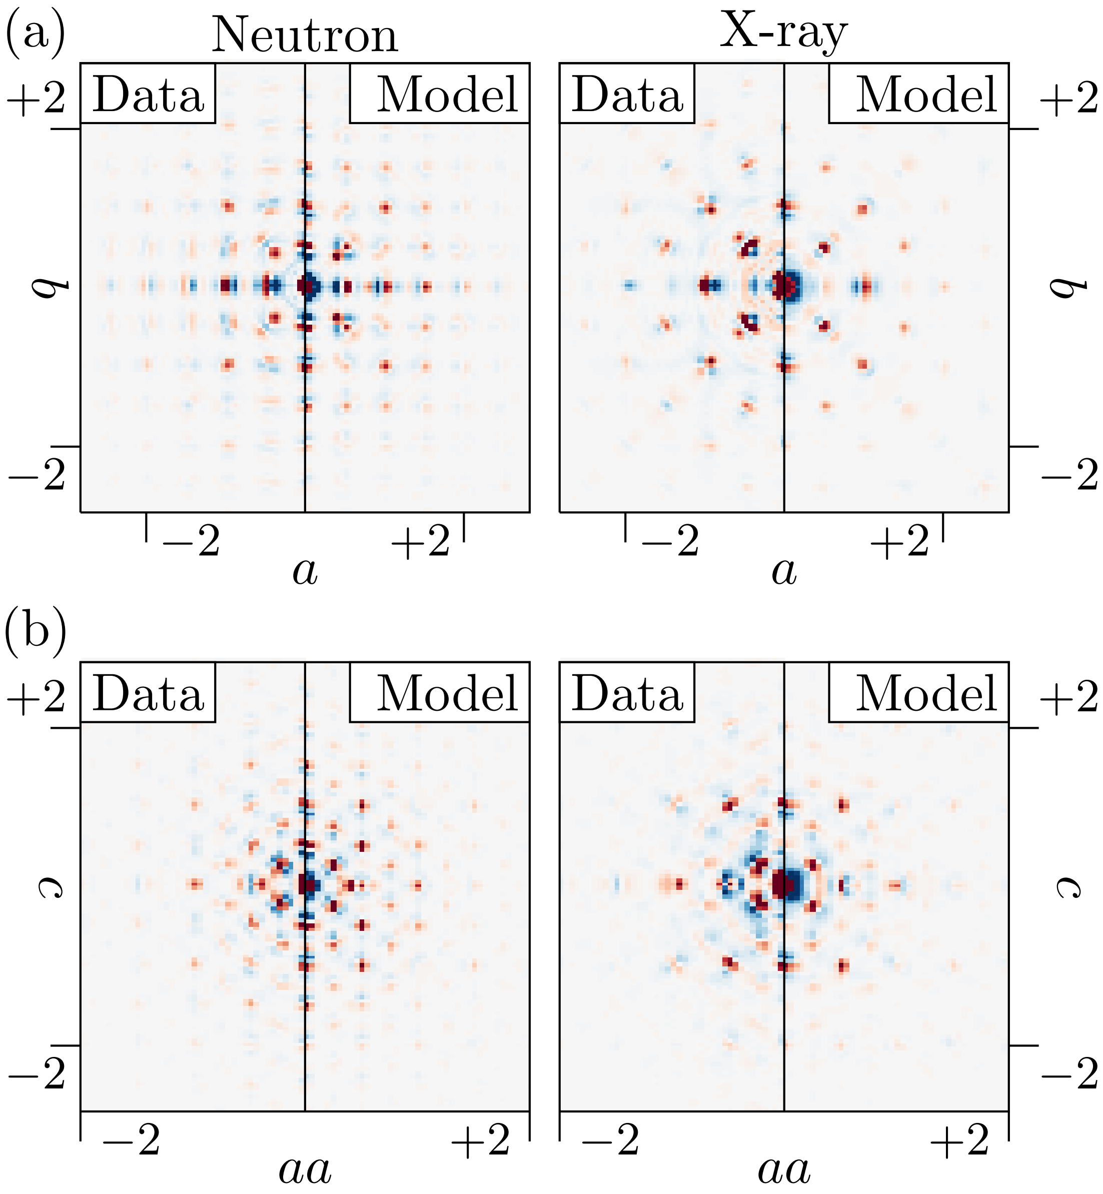


**Figure S4:** 3D-ΔPDF maps of YSZ obtained from neutron (left) and X-ray (right) diffraction experiments compared to the corresponding maps from our model calculations. (a) $ab0$-layer, (b) $aac$-layer. Positive intensities in red, negative intensities in blue.
